# Supplementary material for: Sample Complexity of Uniform Convergence for Multicalibration
Source: arXiv:2005.01757 source file (2021-06-07)
Supplement: Supplementary file 1 [file appendixChernoff.tex]

Throughout this paper, we use the following standard Chernoff bounds.
%%
% Absolute Chernoff Bound
\begin{lemma}[Absolute Chernoff Bound]\label{abs_chernoff_thm}
Let $X_1, ..., X_n$ be i.i.d. binary random variables with $\Ex[X_i] = \mu$ for all $i \in [n]$. Then, for any $\epsilon > 0$:
$\Prob\left[ \left| \frac{1}{n}\sum_{i=1}^{n}{X_i} - \mu \right| \geq \epsilon \right]
\leq
2\exp(-2 \epsilon^2 n)$.
\end{lemma}
%%
% Relative Chernoff Bound
\begin{lemma}[Relative Chernoff Bound]\label{rel_chernoff_thm}
Let $X_1, ..., X_n$ be i.i.d. binary random variables and let $X$ denote their sum. Then, for any $\epsilon \in (0,1)$:$
\Prob\left[ X \leq (1-\epsilon)\Ex[X] \right]
\leq
\exp(-\epsilon^2 \Ex[X]/2)$.
\end{lemma}
